# Supplementary material for: Spontaneous autophoretic motion of isotropic particles
Source: arXiv:1211.6935 ancillary file (2013-06-27)
Supplement: Supplementary file 1 [file SupplementPoF_Revised.pdf]

# Supplemental material for "Spontaneous autophoretic motion of isotropic particles"

Sébastien Michelin,[1] Eric Lauga,[2] and Denis Bartolo[3]
[1) ]*LadHyX – Département de Mécanique, Ecole polytechnique, 91128 Palaiseau Cedex, France*
[2) ]*Department of Mechanical and Aerospace Engineering, University of California San Diego, 9500 Gilman Drive, La Jolla CA 92093-0411, USA.*
[3) ]*Laboratoire de Physique de l'Ecole Normale Supérieure de Lyon, Université de Lyon and CNRS, 46, allée dItalie, F-69007 Lyon, France*

We restrained the analysis in the Letter to a minimal reaction-kinetic model where the reactants are created/destructed with a constant flux regardless of the local solute concentrations. Here we demonstrate that the spontaneous motion is a generic mechanism which applies to more realistic reaction kinetics. We consider a reaction $A \to B$ catalyzed by the surface of the colloid with a constant reaction rate $k$. The approach and methods presented in the paper remain unchanged but for the reactant flux at the surface of the particle. The surface activity now depends on the local concentration of reactant, $D\mathbf{n}\cdot\nabla C_A = kC_A$, at $r = a$. In general, the advection-diffusion of both the products and the reactants must be considered. For simplicity, we consider the case where the interaction of the colloid with $B$ is negligible compared to that with $A$. Following the approach of the paper, the characteristic activity of the colloid is now equal to $\mathcal{A} = -kC_\infty$ (absorption) where $C_\infty$ is the far-field concentration of the reactant. In non-dimensional form, Eqs. (2)–(7) remain unchanged except Eq. (5) which becomes

$$\frac{\partial c}{\partial r}(r=1) = \mathrm{Da}\, c(r=1), \tag{1}$$

where $\mathrm{Da} = ka/D$ is an additional dimensionless number, commonly referred to as the Damköhler number (J. F. Brady *J. Fluid Mech*, **667**, 216, 2010), and is a relative measurement of diffusive and reactive time-scales. The constant flux approximation considered in the Letter corresponds to $\mathrm{Da} = 0$: the reaction is slow compared to diffusion processes and the reactant absorption is controlled by its far-field concentration. The system is now described by two control parameters, the signed Péclet number $\mathrm{Pe} = -k\mathcal{M}aC_\infty/D^2$, and the new number, $\mathrm{Da}$. Considering a perturbation from the isotropic non-swimming state, $\bar{c} = \mathrm{Da}^{-1} - 1/[(1+\mathrm{Da})r]$ and $\bar{\mathbf{u}} = 0$ (a stationary solution of the problem for all Pe and Da), the linear stability analysis identifies again an infinite discrete set of critical Péclet numbers $\mathrm{Pe}_n$ above which the $n$th squirming mode becomes unstable

$$\mathrm{Pe}_1 = 2(1+\mathrm{Da})(2+\mathrm{Da}), \tag{2}$$

$$\mathrm{Pe}_n = 4(n+1+\mathrm{Da})(1+\mathrm{Da}) \quad \text{for} \quad n \geq 2. \tag{3}$$

Consistently with the rest of the paper, self-propulsion can only be achieved by particles with negative mobility ($\mathcal{AM} > 0$). The growth rate of the swimming mode is shown on Fig. 1 (top). The effect of the reaction ($\mathrm{Da} \neq 0$) is to delay the onset of spontaneous swimming and to reduce the instability growth rate (relative to the reaction time-scale). The supercritical nature of the transition is confirmed for all Da using nonlinear simulations. The long-time non-dimensional velocity of the colloid particle is shown on Fig. 1 (bottom), and is always maximum for $\mathrm{Da} = 0$. These results confirm that the self-propulsion mechanism identified in this paper exists for a large class of surface chemical reactions.

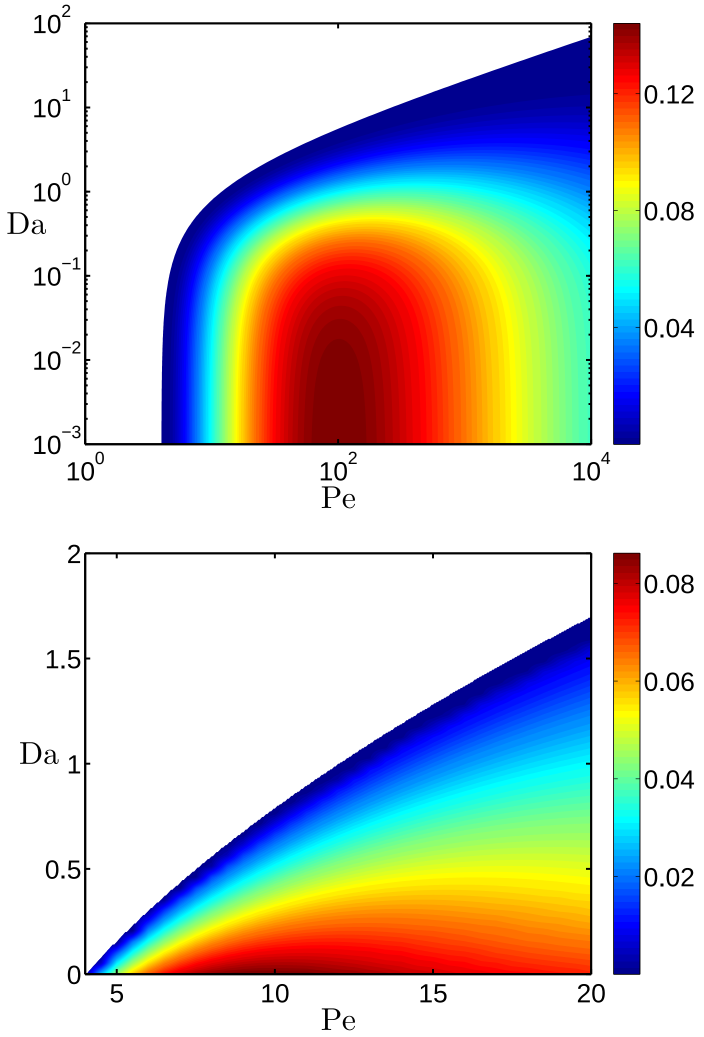


FIG. 1. (Color online) Top: Growth rate of the unstable swimming mode as a function of the Péclet (Pe) and Damköhler (Da) numbers. Bottom: Steady state swimming velocity as a function of Pe and Da.
